# Supplementary material for: Comparing the Robustness of Modern No-Reference Image- and Video-Quality Metrics to Adversarial Attacks
Source: arXiv:2310.06958 source file (2024-02-27)
Supplement: Supplementary file 1 [file Antsiferova_supplementary.pdf]

# Supplementary materials: Comparing the robustness of modern no-reference image- and video-quality metrics to adversarial attacks

**Anastasia Antsiferova**[1,2*], **Khaled Abud**[3*], **Aleksandr Gushchin**[1,2,3*], **Ekaterina Shumitskaya**[3*], **Sergey Lavrushkin**[1,2], **Dmitriy Vatolin**[1,2,3]
[1]MSU Institute for Artificial Intelligence
[2]ISP RAS Research Center for Trusted Artificial Intelligence
[3]Lomonosov Moscow State University
{aantsiferova, khaled.abud, alexander.gushchin, ekaterina.shumitskaya, sergey.lavrushkin, dmitriy}@graphics.cs.msu.ru

## Limitations

This study provides IQA/VQA metrics robustness analysis to the nine popular adversarial attacks. Metrics that are robust to these attacks may appear vulnerable to other existing attacks and newly developed ones. We did not analyse the perceptual quality of attacked images for several reasons. Firstly, our aim was to investigate the general limitations of metrics usage as loss components or as measures in benchmarks. In real-life scenarios, the developers of video codecs or other processing methods would not use extreme attacks that drop down perceptual quality, but it's probable in benchmarking cases. Secondly, according to our knowledge, the intensity of an attack correlates with perceptual quality, which means that reducing the visibility of our attacks will cause general success but will not change the obtained results significantly.

For now, we have not investigated ways to eliminate applied adversarial attacks. However, there are benchmarks of adversarial defences (Croce et al. 2020; rob) created for computer vision tasks. We are working on the release of our own benchmark of defences against adversarial attacks on quality metrics.

This benchmark can be used as a reference to the general robustness of popular IQA/VQA metrics to popular adversarial attacks. However, the robustness may change when you apply different transformations to an attacked image. For example, compression is a way to defend metrics from adversarial attacks (Guo et al. 2017), which means that this leaderboard may change if we compress attacked images in our pipeline. Other transformations may include image super-resolution, deblurring, deblocking, etc. In this study, we did not investigate attacks together with image-processing defence techniques. First of all, there are too many types of them and we consider starting with compression. Secondly, according to our preliminary results with compression of attacked images, its application reduces attacks' success proportionally to its value. It means that if the metric is highly vulnerable, the compression will unlikely remove the attack completely. The same effect may appear with other processing, but now it remains a promising topic for further research.

[*]These authors contributed equally.
Copyright © 2024, Association for the Advancement of Artificial Intelligence (www.aaai.org). All rights reserved.

## Additional experimental details

### Datasets description

For testing, we have used images and video from five datasets:

- **COCO** (Lin et al. 2014) has become a standard benchmark for evaluating and training computer vision algorithms. It has facilitated the development of state-of-the-art models in tasks like object detection, instance segmentation, image captioning, and visual question answering. Its large-scale, diverse, and accurately annotated data make it a valuable resource for advancing the field of computer vision.
- **Pascal VOC 2012** (Everingham et al. 2012) is a widely used benchmark dataset for object recognition and detection tasks in computer vision. It is part of the PASCAL Visual Object Classes (VOC) Challenge, which was organized annually from 2005 to 2012.
- **Vimeo-90k** (Xue et al. 2019) is a large-scale high-quality video dataset for lower-level video processing. It proposes three different video processing tasks: frame interpolation, video denoising/deblocking, and video super-resolution. We used triplets subset that consists of 3-frame sequences with a fixed resolution of $448 \times 256$, extracted from 15K selected video clips from Vimeo-90K. This dataset is designed for temporal frame interpolation.
- **NIPS 2017: Adversarial Learning Development Set** (nip 2017) was organized by Google Brain for Competition on Adversarial Examples and Defenses within the NIPS 2017 competition track. This dataset contains the development images for this competition.
- **Derf's collection (blue_sky video)** (der 2001) is a collection of videos with various content.

The datasets are publicly available and can be acquired by the following links:

- COCO with CC-BY 4.0 license. https://cocodataset.org/#home
- Pascal VOC 2012. http://host.robots.ox.ac.uk/pascal/VOC/
- Vimeo-90k. http://toflow.csail.mit.edu/

- NIPS 2017: Adversarial Learning Development Set. https://www.kaggle.com/datasets/google-brain/nips-2017-adversarial-learning-development-set
- Derf's collection (blue_sky sequence) with no copyright or restrictions on the use. https://media.xiph.org/video/derf/

We used PyAV python library(pya 2023) for splitting the videos into individual frames.

```
import av
container = av.open(path_to_video)
video_stream = container.streams.video
    [0]
frame_array = container.decode(
    video_stream)
```

## Quality assessment methods description

Table 2 lists image and video quality assessment methods used in our experiments. We provide links to original implementations, but the original code was slightly modified to operate within our framework. Method parameters were not changed. All implementations use the PyTorch library, which allows the computation of the gradient of loss w.r.t. input image uniformly for all metrics. All considered quality assessment methods monotonically increase as image/video quality does.

**Analysis of metrics' features that make them stable to adversarial attacks** We summarised implementation details of tested metrics to analyse features that could lead to adversarial robustness in 1. Robust META-IQA uses a relatively small backbone network but efficiently leverages prior knowledge of various image distortions obtained during so-called meta-learning. MDTVSFA metric is the only metric that showed good overall stability and has high correlations with human perception(Antsiferova et al. 2022), and its key features include training on multiple IQA datasets at once. Notably, the CLIP-IQA metric, which adapted CLIP architecture for IQA tasks, shows good resistance to FGSM-based attacks, but the average stability across all attacks is not very high. The worst stability is consistently shown by the FPR metric. It may be caused by its extremely unusual architecture for the NR-IQA task, which includes a Siamese network and an attempt to "hallucinate" the features of the pseudo-reference image from a distorted one.

## Adversarial attacks description

Table 3 contains parameters description for employed adversarial attacks. AMI-FGSM (Sang et al. 2022), Korhonen et al. (Korhonen and You 2022) and MADC (Wang and Simoncelli 2008) did not have original code so we implemented them using algorithms 1, 2, 3. Our implementations are available in *link is hidden for a blind review*. We chose $\epsilon$ equal to $\frac{10}{255}$ for all attacks if applicable because this value is widely used for attacks on classifiers. For iterative attacks we tried different amounts of iterations in the range of 1–100, however, due to the computation complexity we used 1–10 iterations depending on attack success and speed. For UAP attacks training we tried a number of epochs in the range of 1–10 and dataset size in the range of 1,000–10,000. Optimal attack success on validation was reached when 5 iterations and 6,000 dataset size was used (see Figure 1).

**Algorithm 1: AMI-FGSM adversarial attack**

**Inputs:** image $\mathbf{I}$, target quality-metric $\mathbf{M}$,
restriction on $l_p$ norm of the perturbation $\epsilon$,
number of iterations $n_{iters}$
**Output:** adversarial image $I_{adv}$
$I_{adv} = I$
$\alpha = \frac{\epsilon}{n_{iters}}$
$\nu = 1$
$g\_prev = 0$
**for** $i = 1$ to $n_{iters}$ **do**
  $score = \mathbf{M}(\mathbf{I_{adv}})$
  $loss = 1 - \frac{score}{M\_range}$
  {Compute the gradient $g$ with respect to $I_{adv}$}
  $g = g + \nu \cdot g\_prev$
  $g = sign(g)$
  $I_{adv} = I_{adv} - \alpha \cdot g$
**end for**

**Algorithm 2: Korhonen et al. adversarial attack**

**Inputs:** image $\mathbf{I}$, target quality-metric $\mathbf{M}$,
step size $\alpha$, number of iterations $n_{iters}$
**Output:** adversarial image $I_{adv}$
$I_{adv} = I$
$sp\_map = SpatialActivityMap(I)$
**for** $i = 1$ to $n_{iters}$ **do**
  $score = \mathbf{M}(\mathbf{I_{adv}})$
  $loss = 1 - \frac{score}{M\_range}$
  {Compute the gradient $g$ with respect to $I_{adv}$}
  $g = g \cdot sp\_map$
  {Update $I_{adv}$ using optimizer step with $lr = \alpha$}
**end for**

## Evaluation metrics description

We used MinMaxScaler from the preprocessing module of the Scikit-learn library (Pedregosa et al. 2011) to normalize the metric values to the range [0,1]. To calculate Wasserstein- and Energy-distance, the corresponding functions from SciPy's (Virtanen et al. 2020) stats module were used (`wasserstein_distance(x,y)` and `energy_distance(x,y)`). We employed a small neural network consisting of four linear layers as a model for metrics domain transformation, as shown in a one-dimensional example in the repository (NOT 2023). It was trained according to algorithm 4 described in (Korotin, Selikhanovych, and Burnaev 2023) for metric scores on the NIPS 2017 dataset.

# Evaluation pipeline scheme

Fig. 2 visualises the pipeline of our benchmark.

# Additional experimental results

## Results on different test datasets

In the paper, we showed the results combined for all test datasets as they did not differ much between each other. Table 5 contains robustness scores for metrics on NIPS 2017,

| Metric | $R_{score} \uparrow$ | CNN-backbone | Number of params | Train datasets | Input transformations |
|---|---|---|---|---|---|
| META-IQA | 1.168 | ResNet-18 | 13.2M | | ImageNet Normalization |
| NIMA | 1.152 | MobileNetV2 | 2.24M | AVA: 255,000 images | $224 \times 224$ resize |
| MDTVSFA | 0.99 | ResNet-50 | 24.05M | LIVE-VQC, LIVE-Qualcomm, KoNViD-1k, CVD2014 | ImageNet Normalization |
| MANIQA | 0.986 | ViT-B/8 | 135.62M | LIVE, CSIQ, TID2013, KADID-10K, PIPAL | $224 \times 224$ crop |
| WSP | 0.893 | ResNet-101 | 46.7M | Subset of KonIq-10K | |
| RANK-IQA | 0.843 | VGG-16 | 134.26M | | $224 \times 224$ resize |
| HYPER-IQA | 0.740 | ResNet-50 | 27.38M | LIVE, KonIQ-10K, BID, CSIQ | Random cropping, ImageNet Normalization, $224 \times 224$ resize |
| CLIP-IQA | 0.702 | ResNet-50 | | | |
| VSFA | 0.659 | ResNet-50 | 24.06M | KoNViD-1k: 1,000 videos | ImageNet Normalization |
| KONCEPT | 0.584 | InceptionResNetV2 | 59.82M | KonIQ-10k: 10,000 images | Normalization (0.5, 0.5) |
| SPAQ | 0.493 | ResNet-50 | 23.5M | Proposed (11,000 images) | $224 \times 224$ crop |
| PAQ2PIQ | 0.449 | ResNet-18 | 11M | Proposed (40,000 images) | No |
| TRES | 0.320 | ResNet-50 | 152.5M | | |
| LINEARITY | 0.267 | ResNeXt-101 | 90M | KonIQ-10k: 10,000 images | ImageNet Normalization |
| FPR | -0.229 | Custom | 16.6M | TID2013, LIVE, CSIQ, KADID-10k | |

Table 1: Implementation details of evaluated metrics.

VIMEO and “Blue sky” video from Derf’s collection separately. The results on NIPS 2017 and VIMEO datasets are similar, while leaders in stability scores are different for “Blue sky”. This video sequence differs from other datasets for two reasons. First, the resolution is bigger while UAP attacks were trained on a small resolution. Second, the attacks were applied frame-by-frame and all frames within one video sequence are relatively similar while images from other test datasets vary a lot.

### Results for different stability measurement scores

Tables 7, 9, 11, 13 show metrics robustness to all types of tested adversarial attacks by different stability measurement scores. Results are very similar for absolute and relative gain, as well as for energy distance (shown in the main part of the paper) and Wasserstein score. The leaders differ a bit only according to robustness score (Zhang et al. 2022) which is likely caused by its non-linearity (it applies logarithm).

Fig. 3 shows supplemental visualisations for adversarial attacks efficiency depending on SSIM between original and attacked images. The robustness score is averaged within a sliding window of 0.1 (in the main part of the paper, this chart shows results averaged for all examples with SSIM loss that is less or equal to each point on the x-axis). Fig. 4 shows supplemental results for iterative attacks efficiency depending on PSNR loss.

### Results for resistance to UAP attacks trained on different datasets

Table 14 compares metrics robustness to UAP adversarial attacks trained on different datasets (COCO and Pascal VOC). Leaderboard and general stability results are the same. On the one hand, it proves that trained perturbations are stable. On the other hand, these datasets contain images of similar resolution, when perturbation for bigger resolution may be different. Investigating stability to perturbations of bigger resolution is a subject for further research.

### Results without metrics domain transformation

Table 15 shows the results for different stability score measures without domain transformation of metrics. As we described in the paper, we used optimal transport to transfer all metrics’ scales to one (MDTVSFA). We noticed that if we do not apply domain transformation, the leaderboard of tested metrics does not change for all of the robustness scores. In cases when domain transformation is time- or resources-consuming, we assume that this step can be omitted, at least for comparing metrics from our list. Some new metrics may have unusual distributions of values that require transformation for getting correct comparison results.

## Example usage and reproducibility

Code for reproducing our main results is available in the repository *link is hidden for a blind review*. It runs all types of trained attacks for one metric on all available datasets and evaluates its robustness according to our methodology. The

Table 2: Source code to official implementations of quality assessment methods.

| Metric | Year | Image or Video | Implementation |
|---|---|---|---|
| CLIP-IQA (Wang, Chan, and Loy 2023) | 2022 | Image | https://github.com/IceClear/CLIP-IQA |
| META-IQA (Zhu et al. 2020) | 2020 | Image | https://github.com/zhuhancheng/MetaIQA |
| RANK-IQA (Liu, Van De Weijer, and Bagdanov 2017) | 2017 | Image | https://github.com/YunanZhu/Pytorch-TestRankIQA |
| HYPER-IQA (Su et al. 2020) | 2020 | Image | https://github.com/chaofengc/IQA-PyTorch |
| KONCEPT (Hosu et al. 2020) | 2020 | Image | https://github.com/ZhengyuZhao/koniq-PyTorch |
| FPR (Chen et al. 2022) | 2022 | Image | https://github.com/Baoliang93/FPR |
| NIMA (Talebi and Milanfar 2018) | 2018 | Image | https://github.com/truskovskiyk/nima.pytorch/tree/v1 |
| WSP (Su and Korhonen 2020) | 2020 | Image | https://github.com/yichengsu/ICIP2020-WSP-IQA |
| MDTVSFA (Li, Jiang, and Jiang 2021) | 2021 | Video | https://github.com/lidq92/MDTVSFA |
| LINEARITY (Li, Jiang, and Jiang 2020) | 2020 | Image | https://github.com/lidq92/LinearityIQA |
| VSFA (Li, Jiang, and Jiang 2019) | 2019 | Video | https://github.com/lidq92/VSFA |
| PAQ2PIQ (Ying et al. 2020) | 2020 | Image | https://github.com/baidut/paq2piq |
| SPAQ (Fang et al. 2020) | 2020 | Image | https://github.com/h4nwei/SPAQ |
| TRES (Golestaneh, Dadsetan, and Kitani 2022) | 2022 | Image | https://github.com/isalirezag/TReS |
| MANIQA (Yang et al. 2022) | 2022 | Image | https://github.com/IIGROUP/MANIQA |

repository contains several utility files containing primary functions and a demo Jupyter Notebook file which contains an example of launching all the attacks and estimating their results. To reproduce the results, one can simply run all the cells in it sequentially.

We also provide the results of our runs for all the metrics as of this writing. They can be downloaded from *link is hidden for a blind review* as a dataframe in feather format. Pandas.read_feather() can be used to open the file with Python and Pandas library. It contains metrics scores before and after each attack and also SSIM, PSNR and MSE measures between original images and their attacked counterparts.

## References


???? https://ml.cs.tsinghua.edu.cn/adv-bench/#/.

2001. https://media.xiph.org/video/derf/.

2017. https://www.kaggle.com/datasets/google-brain/nips-2017-adversarial-learning\\-development-set.

2023. https://pyav.org/docs/stable/#.

2023. https://github.com/iamalexkorotin/NeuralOptimalTransport.

Antsiferova, A.; Lavrushkin, S.; Smirnov, M.; Gushchin, A.; Vatolin, D.; and Kulikov, D. 2022. Video compression dataset and benchmark of learning-based video-quality metrics. In *Advances in Neural Information Processing Systems*, volume 35, 13814–13825.

Chen, B.; Zhu, L.; Kong, C.; Zhu, H.; Wang, S.; and Li, Z. 2022. No-Reference Image Quality Assessment by Hallucinating Pristine Features. *IEEE Transactions on Image Processing*, 31: 6139–6151.

Croce, F.; Andriushchenko, M.; Sehwag, V.; Debenedetti, E.; Flammarion, N.; Chiang, M.; Mittal, P.; and Hein, M. 2020. RobustBench: a standardized adversarial robustness benchmark. *arXiv preprint arXiv:2010.09670.*

Everingham, M.; Van Gool, L.; Williams, C. K. I.; Winn, J.; and Zisserman, A. 2012. The PASCAL Visual Object Classes Challenge 2012 (VOC2012) Results. http://www.pascal-network.org/challenges/VOC/voc2012/workshop/index.html.

Fang, Y.; Zhu, H.; Zeng, Y.; Ma, K.; and Wang, Z. 2020. Perceptual quality assessment of smartphone photography. In *Proceedings of the IEEE/CVF Conference on Computer Vision and Pattern Recognition*, 3677–3686.

Golestaneh, S. A.; Dadsetan, S.; and Kitani, K. M. 2022.

Table 3: Attacks description, where $\epsilon$ is the restriction on $l_\infty$-norm of adversarial perturbation and $\alpha$ is the step size.

| Attack method | $\epsilon$ | $\alpha$ | $n_{iters}$ | $n_{epochs}$ | Original Implementation |
|---|---|---|---|---|---|
| FGSM | $\frac{10}{255}$ | $\frac{\epsilon}{n_{iters}}$ | 1 | - | https://github.com/1Konny/FGSM |
| I-FGSM | $\frac{10}{255}$ | $\frac{\epsilon}{n_{iters}}$ | 10 | - | https://github.com/1Konny/FGSM |
| MIFGSM | $\frac{10}{255}$ | $\frac{\epsilon}{n_{iters}}$ | 10 | - | https://github.com/Harry24k/adversarial-attacks-pytorch |
| AMI-FGSM | $\frac{10}{255}$ | $\frac{\epsilon}{n_{iters}}$ | 10 | - | Implementation described in algorithm 1 Description from paper (Sang et al. 2022) |
| Optimised-UAP | $\frac{25}{255}$ | - | - | 5 | https://github.com/katiashh/UAP_Attack_on_Quality_Metrics |
| Cumulative-UAP | $\frac{25}{255}$ | - | - | 5 | https://github.com/BXuan694/Universal-Adversarial-Perturbation |
| Generative-UAP | $\frac{10}{255}$ | - | - | 1 | Adaptation of code from https://github.com/OmidPoursaeed/Generative_Adversarial_Perturbations |
| Korhonen et al. | - | 0.005 | 10 | - | Implementation described in algorithm 2 Description from paper (Korhonen and You 2022) |
| MADC | $\frac{10}{255}$ | 0.001 | 8 | - | Implementation described in algorithm 3 Description from paper (Wang and Simoncelli 2008) |

Algorithm 3: MADC adversarial attack

**Inputs:** image $\mathbf{I}$, target quality-metric $\mathbf{M}$,
restriction on $l_p$ norm of the perturbation $\epsilon$, step size $\alpha$
number of iterations $n_{iters}$
**Output:** adversarial image $I_{adv}$
$I_{adv} = I$
**for** $i = 1$ to $n_{iters}$ **do**
  $score = \mathbf{M}(\mathbf{I_{adv}})$
  $loss = 1 - \frac{score}{M\_range}$
  {Compute the gradient $g1$ with respect to $I_{adv}$}
  $loss = \sqrt{mean((I_{adv} - I)^2)}$
  {Compute the gradient $g2$ with respect to $I_{adv}$}
  $pg = g1 - \frac{g2^T \cdot g1}{g2^T \cdot g2} \cdot g2$
  $pg = sign(pg)$
  $I_{adv} = I_{adv} - \alpha \cdot pg$
  $cur\_norm = \sqrt{mean((I_{adv} - I)^2)}$
  **while** $cur\_norm > \epsilon$ **do**
    {Compute the gradient $g2$ with respect to $I_{adv}$}
    $g2 = sign(g2)$
    $I_{adv} = I_{adv} - 0.0005 \cdot g2$
    $cur\_norm = \sqrt{mean((I_{adv} - I)^2)}$
  **end while**
**end for**


No-reference image quality assessment via transformers, relative ranking, and self-consistency. In *Proceedings of the IEEE/CVF Winter Conference on Applications of Computer Vision*, 1220–1230.

Guo, C.; Rana, M.; Cisse, M.; and Maaten, L. 2017. Countering Adversarial Images using Input Transformations.

Hosu, V.; Lin, H.; Sziranyi, T.; and Saupe, D. 2020. KonIQ-10k: An ecologically valid database for deep learning of blind image quality assessment. *IEEE Transactions on Image Processing*, 29: 4041–4056.

Korhonen, J.; and You, J. 2022. Adversarial Attacks Against Blind Image Quality Assessment Models. In *Proceedings of the 2nd Workshop on Quality of Experience in Visual Multimedia Applications*, 3–11.

Korotin, A.; Selikhanovych, D.; and Burnaev, E. 2023. Neural Optimal Transport. In *International Conference on Learning Representations*.

Li, D.; Jiang, T.; and Jiang, M. 2019. Quality assessment of in-the-wild videos. In *Proceedings of the 27th ACM International Conference on Multimedia*, 2351–2359.

Li, D.; Jiang, T.; and Jiang, M. 2020. Norm-in-norm loss with faster convergence and better performance for image quality assessment. In *Proceedings of the 28th ACM International Conference on Multimedia*, 789–797.

Li, D.; Jiang, T.; and Jiang, M. 2021. Unified quality assessment of in-the-wild videos with mixed datasets training. *International Journal of Computer Vision*, 129: 1238–1257.

Lin, T.-Y.; Maire, M.; Belongie, S.; Hays, J.; Perona, P.; Ramanan, D.; Dollár, P.; and Zitnick, C. L. 2014. Microsoft coco: Common objects in context. In *Computer Vision–ECCV 2014: 13th European Conference, Zurich, Switzerland, September 6-12, 2014, Proceedings, Part V 13*, 740–755. Springer.

Liu, X.; Van De Weijer, J.; and Bagdanov, A. D. 2017. Rankiqa: Learning from rankings for no-reference image quality assessment. In *Proceedings of the IEEE international conference on computer vision*, 1040–1049.

Pedregosa, F.; Varoquaux, G.; Gramfort, A.; Michel, V.; Thirion, B.; Grisel, O.; Blondel, M.; Prettenhofer, P.; Weiss, R.; Dubourg, V.; et al. 2011. Scikit-learn: Machine learning in Python. *Journal of machine learning research*, 12(Oct): 2825–2830.

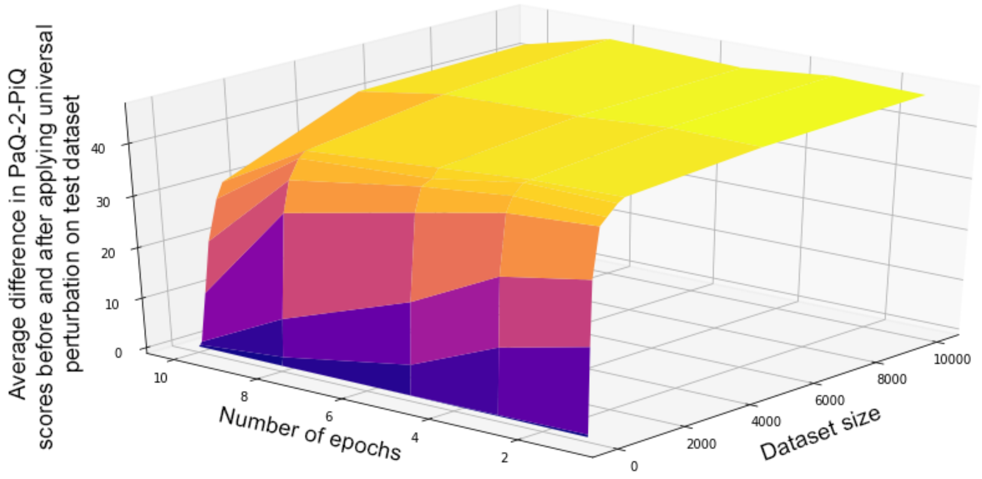


Figure 1: Visualization of experimental search for optimal hyper-parameters (number of epochs and dataset size) for Optimized UAP attack when attacking PaQ-2-PiQ NR quality metric.

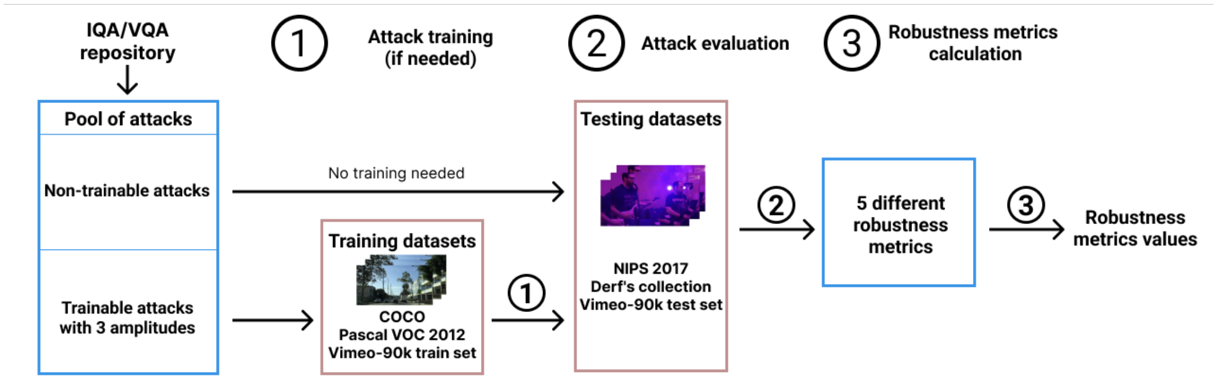


Figure 2: Evaluation pipeline scheme.

Sang, Q.; Zhang, H.; Liu, L.; Wu, X.; and Bovik, A. 2022. On the Generation of Adversarial Samples for Image Quality Assessment. *Available at SSRN 4112969*.

Su, S.; Yan, Q.; Zhu, Y.; Zhang, C.; Ge, X.; Sun, J.; and Zhang, Y. 2020. Blindly assess image quality in the wild guided by a self-adaptive hyper network. In *Proceedings of the IEEE/CVF Conference on Computer Vision and Pattern Recognition*, 3667–3676.

Su, Y.; and Korhonen, J. 2020. Blind natural image quality prediction using convolutional neural networks and weighted spatial pooling. In *2020 IEEE International Conference on Image Processing (ICIP)*, 191–195. IEEE.

Talebi, H.; and Milanfar, P. 2018. NIMA: Neural image assessment. *IEEE transactions on image processing*, 27(8): 3998–4011.

Virtanen, P.; Gommers, R.; Oliphant, T. E.; Haberland, M.; Reddy, T.; Cournapeau, D.; Burovski, E.; Peterson, P.; Weckesser, W.; Bright, J.; van der Walt, S. J.; Brett, M.; Wilson, J.; Millman, K. J.; Mayorov, N.; Nelson, A. R. J.; Jones, E.; Kern, R.; Larson, E.; Carey, C. J.; Polat, İ.; Feng, Y.; Moore, E. W.; VanderPlas, J.; Laxalde, D.; Perktold, J.; Cimrman, R.; Henriksen, I.; Quintero, E. A.; Harris, C. R.; Archibald, A. M.; Ribeiro, A. H.; Pedregosa, F.; van Mulbregt, P.; and SciPy 1.0 Contributors. 2020. SciPy 1.0: Fundamental Algorithms for Scientific Computing in Python. *Nature Methods*, 17: 261–272.

Wang, J.; Chan, K. C.; and Loy, C. C. 2023. Exploring CLIP for Assessing the Look and Feel of Images. In *AAAI*.

Wang, Z.; and Simoncelli, E. P. 2008. Maximum differentiation (MAD) competition: A methodology for comparing computational models of perceptual quantities. *Journal of Vision*, 8(12): 8–8.

Xue, T.; Chen, B.; Wu, J.; Wei, D.; and Freeman, W. T. 2019. Video Enhancement with Task-Oriented Flow. *International Journal of Computer Vision (IJCV)*, 127(8): 1106–1125.

Yang, S.; Wu, T.; Shi, S.; Lao, S.; Gong, Y.; Cao, M.; Wang,

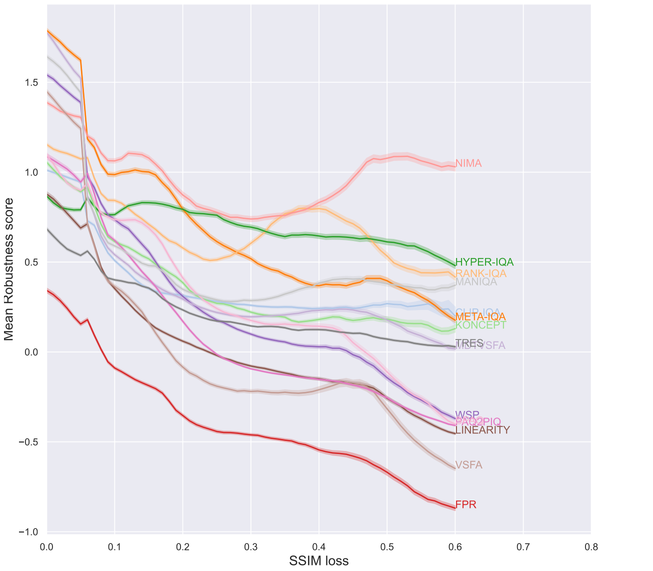


Figure 3: Dependency of metrics robustness scores on SSIM loss averaged in a 0.1 sliding window for attacked images (all types of attacks).

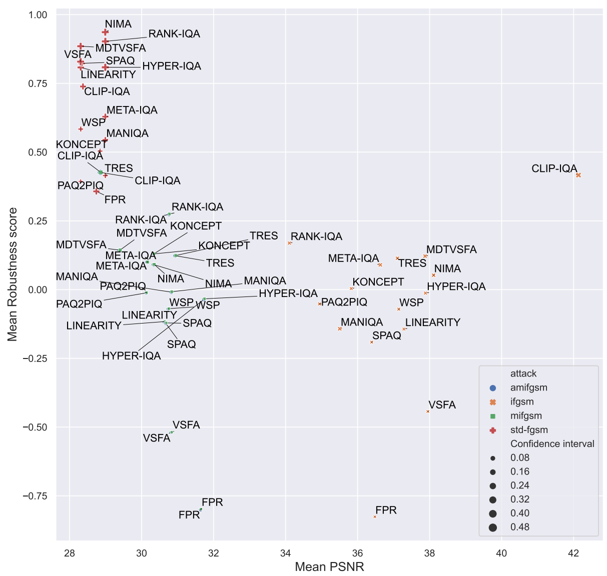


Figure 4: Mean robustness score of compared metrics versus mean PSNR for iterative attacks.


J.; and Yang, Y. 2022. Maniqa: Multi-dimension attention network for no-reference image quality assessment. In *Proceedings of the IEEE/CVF Conference on Computer Vision and Pattern Recognition*, 1191–1200.

Ying, Z.; Niu, H.; Gupta, P.; Mahajan, D.; Ghadiyaram, D.; and Bovik, A. 2020. From patches to pictures (PaQ-2-PiQ): Mapping the perceptual space of picture quality. In *Proceedings of the IEEE/CVF Conference on Computer Vision and Pattern Recognition*, 3575–3585.

Zhang, W.; Li, D.; Min, X.; Zhai, G.; Guo, G.; Yang, X.; and Ma, K. 2022. Perceptual Attacks of No-Reference Image Quality Models with Human-in-the-Loop. *arXiv preprint arXiv:2210.00933*.

Zhu, H.; Li, L.; Wu, J.; Dong, W.; and Shi, G. 2020. MetaIQA: Deep meta-learning for no-reference image quality assessment. In *Proceedings of the IEEE/CVF Conference on Computer Vision and Pattern Recognition*, 14143–14152.

Algorithm 4: Results evaluation algorithm

**Inputs:** metric scores before the attack $X_{clear}$ and after $X_{attacked}$ (vectors of length $N$), trained domain transformation model $T(.)$. (Training algorithm is described in (Korotin, Selikhanovych, and Burnaev 2023) (Algorithm 1))

**Output:** calculated scores $Abs.gain$, $Rel.gain$, $R_{score}$, $E_{score}$ and $W_{score}$.

$\hat{X}_{clear} = T(X_{clear})$ {Apply N.O.T. domain transformation}
$\hat{X}_{attacked} = T(X_{attacked})$ {Scale to range $[0, 1]$}
$\hat{X}_{clear} = (\hat{X}_{clear} - min(\hat{X}_{clear}))/(max(\hat{X}_{clear}) - min(\hat{X}_{clear}))$
$\hat{X}_{attacked} = (\hat{X}_{attacked} - min(\hat{X}_{clear}))/(max(\hat{X}_{clear}) - min(\hat{X}_{clear}))$
{Evaluate}
$S_{abs} = 0$
$S_{rel} = 0$
$S_R = 0$
**for** $i = 1$ to $N$ **do**
  $S_{abs} += \hat{X}_{i,attacked} - \hat{X}_{i,clear}$
  $S_{rel} += (\hat{X}_{i,attacked} - \hat{X}_{i,clear})/(\hat{X}_{i,clear} + 1)$
  $S_R += log_{10}(max\{1 - \hat{X}_{i,attacked}, \hat{X}_{i,clear}\}/|\hat{X}_{i,attacked} - \hat{X}_{i,clear}|)$
**end for**
$Abs.gain = \frac{1}{N}\sum_{i=1}^{N} S_{abs}$
$Rel.gain = \frac{1}{N}\sum_{i=1}^{N} S_{rel}$
$R_{score} = \frac{1}{N}\sum_{i=1}^{N} S_R$

$W_{score} = sign(\frac{1}{N}\sum_{i=1}^{N} \hat{X}_{i,attacked} - \frac{1}{N}\sum_{i=1}^{N} \hat{X}_{i,clear}) \cdot wasserstein\_distance(\hat{X}_{clear}, \hat{X}_{attacked})$
$E_{score} = sign(\frac{1}{N}\sum_{i=1}^{N} \hat{X}_{i,attacked} - \frac{1}{N}\sum_{i=1}^{N} \hat{X}_{i,clear}) \cdot energy\_distance(\hat{X}_{clear}, \hat{X}_{attacked})$
**return** $Abs.gain, Rel.gain, R_{score}, W_{score}, E_{score}$

| NIPS 2017 dataset, with domain transform, Energy score | | | | | | | | | |
|---|---|---|---|---|---|---|---|---|---|
| Attack | Optimized-UAP | | | Generative-UAP | | | Cumulative-UAP | | |
| Amplitude | 0.2 | 0.4 | 0.8 | 0.2 | 0.4 | 0.8 | 0.2 | 0.4 | 0.8 |
| CLIP-IQA | 0.164 | 0.513 | 0.700 | 0.083 | 0.363 | 0.653 | 0.025 | 0.096 | 0.241 |
| META-IQA | -0.021 | 0.187 | 0.638 | -0.019 | -0.015 | 0.180 | 0.002 | 0.003 | 0.007 |
| RANK-IQA | 0.114 | 0.522 | 0.811 | 0.019 | 0.187 | 0.568 | 0.095 | 0.354 | 0.604 |
| HYPER-IQA | -0.137 | 0.049 | 0.237 | **-0.075** | -0.074 | 0.079 | **-0.104** | 0.043 | 0.289 |
| KONCEPT | 0.092 | 0.499 | 0.968 | -0.014 | 0.248 | 0.627 | 0.144 | 0.489 | 0.841 |
| FPR | 0.816 | 1.945 | 4.502 | 0.329 | 0.862 | 1.684 | 0.392 | 1.091 | 2.928 |
| NIMA | 0.009 | 0.019 | 0.089 | 0.022 | 0.058 | 0.110 | 0.011 | 0.029 | 0.058 |
| WSP | 0.094 | 0.447 | 0.961 | 0.033 | 0.082 | 0.275 | 0.003 | 0.008 | 0.018 |
| MDTVSFA | 0.130 | 0.463 | 0.760 | 0.027 | 0.194 | 0.459 | 0.002 | 0.005 | 0.010 |
| LINEARITY | 0.243 | 0.724 | 1.284 | -0.012 | 0.236 | 0.598 | 0.221 | 0.684 | 1.234 |
| VSFA | 0.161 | 0.686 | 1.513 | 0.029 | 0.188 | 0.506 | 0.003 | 0.012 | 0.042 |
| PAQ2PIQ | 0.170 | 0.781 | 1.374 | 0.012 | 0.176 | 0.671 | 0.139 | 0.705 | 1.287 |
| SPAQ | -0.079 | 0.030 | 0.508 | 0.022 | 0.123 | 0.424 | -0.082 | **-0.045** | 0.476 |
| TRES | 0.336 | 0.667 | 0.953 | 0.104 | 0.340 | 0.679 | 0.296 | 0.631 | 0.914 |
| MANIQA | **-0.185** | **-0.394** | **-0.607** | -0.062 | **-0.167** | **-0.301** | -0.002 | 0.002 | **0.006** |

| VIMEO dataset, with domain transform, Energy score | | | | | | | | | |
|---|---|---|---|---|---|---|---|---|---|
| Attack | Optimized-UAP | | | Generative-UAP | | | Cumulative-UAP | | |
| Amplitude | 0.2 | 0.4 | 0.8 | 0.2 | 0.4 | 0.8 | 0.2 | 0.4 | 0.8 |
| CLIP-IQA | 0.173 | 0.678 | 0.811 | 0.006 | 0.445 | 0.765 | 0.019 | 0.059 | 0.175 |
| META-IQA | -0.035 | 0.241 | 0.795 | -0.026 | -0.030 | 0.227 | 0.002 | 0.004 | 0.008 |
| RANK-IQA | -0.140 | 0.248 | 0.604 | -0.063 | -0.077 | 0.267 | 0.019 | 0.137 | 0.367 |
| HYPER-IQA | -0.196 | 0.148 | 0.417 | **-0.114** | -0.112 | 0.205 | **-0.130** | 0.164 | 0.499 |
| KONCEPT | 0.071 | 0.519 | 1.034 | -0.029 | 0.230 | 0.705 | 0.108 | 0.525 | 0.948 |
| FPR | 0.939 | 1.923 | 3.379 | 0.348 | 0.998 | 1.737 | 0.462 | 1.112 | 1.951 |
| NIMA | -0.033 | -0.039 | 0.043 | 0.021 | 0.054 | 0.134 | 0.007 | 0.018 | 0.035 |
| WSP | 0.254 | 0.970 | 1.629 | 0.083 | 0.204 | 0.578 | 0.004 | 0.014 | 0.039 |
| MDTVSFA | 0.490 | 0.899 | 1.042 | 0.085 | 0.475 | 0.799 | 0.002 | 0.006 | 0.013 |
| LINEARITY | 0.639 | 1.248 | 1.753 | 0.069 | 0.577 | 1.019 | 0.583 | 1.185 | 1.682 |
| VSFA | 0.512 | 1.510 | 2.469 | 0.077 | 0.508 | 1.075 | 0.004 | 0.018 | 0.052 |
| PAQ2PIQ | 0.318 | 1.072 | 1.559 | -0.009 | 0.292 | 0.938 | 0.284 | 1.002 | 1.479 |
| SPAQ | 0.107 | 1.227 | 2.586 | 0.120 | 0.660 | 1.349 | 0.075 | 1.154 | 2.568 |
| TRES | 0.415 | 0.739 | 1.010 | 0.136 | 0.397 | 0.725 | 0.341 | 0.683 | 0.962 |
| MANIQA | **-0.246** | **-0.491** | **-0.671** | -0.087 | **-0.229** | **-0.428** | -0.002 | **-0.006** | **-0.005** |

| "Blue sky" video from Derf's collection, with domain transform, Energy score | | | | | | | | | |
|---|---|---|---|---|---|---|---|---|---|
| Attack | Optimized-UAP | | | Generative-UAP | | | Cumulative-UAP | | |
| Amplitude | 0.2 | 0.4 | 0.8 | 0.2 | 0.4 | 0.8 | 0.2 | 0.4 | 0.8 |
| CLIP-IQA | 1.780 | 3.290 | 3.679 | 0.711 | 1.886 | 2.968 | 0.083 | 0.400 | 1.191 |
| META-IQA | -0.318 | -0.498 | -0.671 | -0.102 | -0.242 | -0.365 | -0.009 | -0.011 | -0.018 |
| RANK-IQA | -0.530 | -0.621 | 0.277 | -0.204 | -0.469 | -0.762 | -0.137 | -0.317 | -0.601 |
| HYPER-IQA | **-1.010** | **-1.511** | **-2.017** | **-0.397** | **-0.840** | **-1.243** | **-0.861** | **-1.337** | **-1.818** |
| KONCEPT | -0.342 | -0.320 | -0.170 | -0.180 | -0.292 | -0.128 | -0.141 | 0.168 | 0.466 |
| FPR | 1.625 | 3.194 | 5.420 | 0.476 | 1.700 | 3.079 | 0.790 | 1.670 | 2.606 |
| NIMA | -0.236 | -0.320 | -0.501 | -0.215 | -0.294 | -0.348 | -0.045 | -0.129 | -0.247 |
| WSP | 1.699 | 2.948 | 3.565 | 0.267 | 0.832 | 1.993 | 0.038 | 0.104 | 0.218 |
| MDTVSFA | 1.381 | 2.062 | 2.222 | 0.162 | 0.785 | 1.525 | 0.007 | 0.007 | 0.019 |
| LINEARITY | 2.764 | 3.661 | 4.380 | 0.977 | 2.500 | 3.261 | 2.655 | 3.570 | 4.292 |
| VSFA | 2.930 | 5.229 | 7.133 | 0.392 | 2.331 | 3.966 | -0.021 | 0.089 | 0.358 |
| PAQ2PIQ | 1.211 | 2.004 | 2.426 | -0.008 | 1.002 | 1.795 | 1.083 | 1.872 | 2.281 |
| SPAQ | -0.568 | -0.726 | -0.875 | -0.215 | -0.376 | -0.300 | -0.577 | -0.732 | -0.871 |
| TRES | 0.436 | 1.047 | 1.578 | 0.076 | 0.368 | 0.857 | 0.216 | 0.816 | 1.415 |
| MANIQA | -0.539 | -1.168 | -1.606 | -0.147 | -0.539 | -1.137 | -0.009 | -0.010 | -0.062 |

Table 4: Robustness scores for tested metrics on different datasets. Table 1

| NIPS 2017 dataset, with domain transform, Energy score | | | | | | |
|---|---|---|---|---|---|---|
| Attack | FGSM | I-FGSM | MI-FGSM | AMI-FGSM | MADC | Korhonen et al. |
| CLIP-IQA | 0.433 | **0.795** | **0.780** | **0.780** | 0.792 | <u>0.787</u> |
| META-IQA | 0.574 | 1.236 | 1.212 | 1.214 | 0.796 | 0.975 |
| RANK-IQA | 0.457 | <u>1.145</u> | <u>0.967</u> | <u>0.968</u> | **0.448** | 0.887 |
| HYPER-IQA | **-0.290** | 1.325 | 1.351 | 1.359 | 0.767 | 1.310 |
| KONCEPT | 0.557 | 1.200 | 1.014 | 1.014 | 0.670 | 1.001 |
| FPR | 0.947 | 3.389 | 3.274 | 3.276 | 1.523 | 3.179 |
| NIMA | 0.383 | 1.326 | 1.261 | 1.263 | 1.056 | 1.203 |
| WSP | 0.457 | 1.289 | 1.270 | 1.275 | 0.711 | 0.962 |
| MDTVSFA | <u>0.259</u> | <u>0.938</u> | <u>0.902</u> | <u>0.902</u> | 0.800 | **0.762** |
| LINEARITY | <u>-0.158</u> | 1.369 | 1.335 | 1.341 | 0.802 | 1.336 |
| VSFA | 0.404 | 2.091 | 2.276 | 2.275 | 1.347 | 1.579 |
| PAQ2PIQ | 0.658 | 1.282 | 1.212 | 1.216 | <u>0.503</u> | 1.088 |
| SPAQ | 0.294 | 1.452 | 1.332 | 1.336 | 0.730 | 1.318 |
| TRES | 0.807 | 1.206 | 1.188 | 1.190 | 0.668 | 1.164 |
| MANIQA | 0.530 | 1.331 | 1.166 | 1.167 | <u>0.619</u> | <u>0.836</u> |

| VIMEO dataset, with domain transform, Energy score | | | | | | |
|---|---|---|---|---|---|---|
| Attack | FGSM | I-FGSM | MI-FGSM | AMI-FGSM | MADC | Korhonen et al. |
| CLIP-IQA | 0.411 | **0.840** | **0.829** | **0.824** | 0.833 | <u>0.830</u> |
| META-IQA | 0.544 | 1.402 | 1.379 | 1.379 | 1.059 | 1.101 |
| RANK-IQA | 0.196 | <u>1.113</u> | <u>0.941</u> | <u>0.944</u> | **0.394** | **0.774** |
| HYPER-IQA | **-0.561** | 1.496 | 1.538 | 1.552 | 0.979 | 1.472 |
| KONCEPT | 0.660 | 1.390 | 1.203 | 1.201 | 0.882 | 1.182 |
| FPR | 0.649 | 3.766 | 3.600 | 3.602 | 2.055 | 3.419 |
| NIMA | 0.183 | 1.197 | 1.143 | 1.142 | 0.966 | 1.026 |
| WSP | 0.485 | 1.404 | 1.381 | 1.385 | 0.871 | 1.026 |
| MDTVSFA | <u>0.170</u> | <u>1.055</u> | <u>1.026</u> | <u>1.026</u> | 0.976 | <u>0.911</u> |
| LINEARITY | <u>-0.298</u> | 1.388 | 1.325 | 1.325 | 0.927 | 1.304 |
| VSFA | 0.321 | 2.267 | 2.508 | 2.507 | 1.709 | 1.821 |
| PAQ2PIQ | 0.596 | 1.262 | 1.192 | 1.187 | <u>0.589</u> | 1.046 |
| SPAQ | 0.351 | 1.956 | 1.762 | 1.769 | 1.023 | 1.701 |
| TRES | 0.831 | 1.233 | 1.221 | 1.222 | <u>0.763</u> | 1.172 |
| MANIQA | 0.622 | 1.651 | 1.436 | 1.438 | 0.869 | 1.026 |

| "Blue sky" video from Derf's collection, with domain transform, Energy score | | | | | | |
|---|---|---|---|---|---|---|
| Attack | FGSM | I-FGSM | MI-FGSM | AMI-FGSM | MADC | Korhonen et al. |
| CLIP-IQA | 2.016 | 3.719 | 3.764 | 3.642 | 3.643 | 3.531 |
| META-IQA | 1.086 | 2.372 | 2.308 | 2.321 | 1.662 | <u>1.566</u> |
| RANK-IQA | 1.119 | <u>2.337</u> | **1.923** | <u>1.971</u> | **1.184** | 1.749 |
| HYPER-IQA | **0.428** | 3.133 | 3.161 | 3.141 | 1.925 | 2.874 |
| KONCEPT | 1.345 | 2.530 | <u>2.039</u> | **1.928** | 1.504 | 1.785 |
| FPR | 2.044 | 8.405 | 8.212 | 8.173 | 4.463 | 6.615 |
| NIMA | 1.830 | 3.655 | 3.476 | 3.476 | 2.649 | 2.927 |
| WSP | 0.982 | 2.784 | 2.962 | 2.947 | 2.315 | 1.959 |
| MDTVSFA | <u>0.547</u> | <u>2.295</u> | 2.295 | 2.283 | 2.192 | **1.218** |
| LINEARITY | 1.060 | 3.684 | 3.355 | 3.369 | 2.894 | 3.335 |
| VSFA | 0.731 | 6.786 | 7.871 | 8.059 | 5.356 | 2.682 |
| PAQ2PIQ | 1.360 | **2.247** | <u>2.179</u> | <u>2.171</u> | <u>1.324</u> | 1.806 |
| SPAQ | 1.058 | 2.666 | 2.508 | 2.499 | 1.452 | 2.025 |
| TRES | 1.868 | 2.834 | 2.785 | 2.747 | 1.894 | 2.713 |
| MANIQA | <u>0.559</u> | 2.510 | 2.241 | 2.325 | <u>1.377</u> | <u>1.239</u> |

Table 5: Robustness scores for tested metrics on different datasets. Table 2

| Attack<br>Amplitude | Optimized-UAP<br>0.2 | <br>0.4 | <br>0.8 | Generative-UAP<br>0.2 | <br>0.4 | <br>0.8 | Cumulative-UAP<br>0.2 | <br>0.4 | <br>0.8 |
|---|---|---|---|---|---|---|---|---|---|
| CLIP-IQA | 0.107<br>(0.104, 0.110) | 0.377<br>(0.371, 0.382) | 0.456<br>(0.451, 0.462) | 0.021<br>(0.018, 0.023) | 0.240<br>(0.236, 0.243) | 0.416<br>(0.412, 0.421) | 0.011<br>(0.011, 0.012) | 0.041<br>(0.040, 0.042) | 0.116<br>(0.114, 0.118) |
| META-IQA | -0.020<br>(-0.022, -0.018) | 0.110<br>(0.105, 0.115) | 0.451<br>(0.442, 0.459) | -0.013<br>(-0.014, -0.013) | -0.016<br>(-0.018, -0.015) | 0.104<br>(0.100, 0.108) | 0.001<br>(0.001, 0.001) | 0.001<br>(0.001, 0.002) | 0.004<br>(0.003, 0.004) |
| RANK-IQA | -0.021<br>(-0.023, -0.019) | 0.149<br>(0.145, 0.153) | 0.342<br>(0.337, 0.347) | -0.018<br>(-0.019, -0.017) | 0.014<br>(0.012, 0.016) | 0.157<br>(0.153, 0.160) | 0.014<br>(0.013, 0.015) | 0.090<br>(0.088, 0.093) | 0.192<br>(0.188, 0.196) |
| HYPER-IQA | -0.086<br>(-0.088, -0.084) | 0.021<br>(0.017, 0.025) | 0.149<br>(0.143, 0.155) | **-0.052**<br>(-0.053, -0.051) | -0.046<br>(-0.048, -0.045) | 0.065<br>(0.061, 0.069) | **-0.057**<br>(-0.059, -0.056) | 0.037<br>(0.034, 0.041) | 0.191<br>(0.185, 0.197) |
| KONCEPT | 0.030<br>(0.028, 0.032) | 0.241<br>(0.236, 0.246) | 0.594<br>(0.586, 0.601) | -0.011<br>(-0.012, -0.010) | 0.104<br>(0.101, 0.108) | 0.342<br>(0.337, 0.348) | 0.052<br>(0.049, 0.054) | 0.245<br>(0.241, 0.250) | 0.501<br>(0.495, 0.506) |
| FPR | 0.621<br>(0.606, 0.636) | 2.502<br>(2.452, 2.552) | 7.970<br>(7.833, 8.107) | 0.146<br>(0.143, 0.149) | 0.665<br>(0.652, 0.679) | 1.836<br>(1.807, 1.865) | 0.218<br>(0.211, 0.224) | 1.093<br>(1.059, 1.127) | 3.657<br>(3.556, 3.759) |
| NIMA | -0.010<br>(-0.012, -0.009) | -0.008<br>(-0.011, -0.006) | 0.022<br>(0.019, 0.025) | 0.005<br>(0.004, 0.006) | 0.022<br>(0.021, 0.024) | 0.057<br>(0.055, 0.06) | 0.004<br>(0.003, 0.004) | 0.011<br>(0.010, 0.012) | 0.021<br>(0.019, 0.022) |
| WSP | 0.129<br>(0.125, 0.134) | 0.595<br>(0.585, 0.606) | 1.288<br>(1.273, 1.302) | 0.033<br>(0.032, 0.034) | 0.086<br>(0.084, 0.088) | 0.269<br>(0.264, 0.275) | 0.002<br>(0.002, 0.002) | 0.006<br>(0.006, 0.007) | 0.017<br>(0.016, 0.017) |
| MDTVSFA | 0.216<br>(0.211, 0.222) | 0.461<br>(0.455, 0.467) | 0.586<br>(0.581, 0.591) | 0.034<br>(0.032, 0.035) | 0.201<br>(0.197, 0.205) | 0.380<br>(0.375, 0.385) | 0.001<br>(0.001, 0.001) | 0.003<br>(0.002, 0.003) | 0.006<br>(0.005, 0.006) |
| LINEARITY | 0.333<br>(0.325, 0.340) | 0.859<br>(0.847, 0.871) | 1.500<br>(1.486, 1.513) | 0.032<br>(0.030, 0.034) | 0.281<br>(0.275, 0.287) | 0.591<br>(0.583, 0.599) | 0.296<br>(0.289, 0.303) | 0.786<br>(0.775, 0.798) | 1.393<br>(1.380, 1.406) |
| VSFA | 0.281<br>(0.273, 0.290) | 1.247<br>(1.225, 1.269) | 2.622<br>(2.597, 2.647) | 0.030<br>(0.028, 0.032) | 0.246<br>(0.240, 0.252) | 0.662<br>(0.651, 0.672) | 0.002<br>(0.001, 0.002) | 0.008<br>(0.007, 0.008) | 0.025<br>(0.024, 0.027) |
| PAQ2PIQ | 0.161<br>(0.156, 0.165) | 0.662<br>(0.654, 0.671) | 1.204<br>(1.195, 1.213) | -0.000<br>(-0.001, 0.000) | 0.136<br>(0.132, 0.139) | 0.520<br>(0.514, 0.527) | 0.136<br>(0.132, 0.140) | 0.581<br>(0.574, 0.589) | 1.088<br>(1.080, 1.097) |
| SPAQ | 0.007<br>(0.005, 0.010) | 0.519<br>(0.503, 0.534) | 1.797<br>(1.761, 1.832) | 0.030<br>(0.029, 0.031) | 0.206<br>(0.200, 0.212) | 0.580<br>(0.569, 0.591) | -0.002<br>(-0.005, -0.0) | 0.462<br>(0.448, 0.477) | 1.772<br>(1.736, 1.807) |
| TRES | 0.203<br>(0.200, 0.206) | 0.403<br>(0.399, 0.407) | 0.631<br>(0.626, 0.635) | 0.065<br>(0.064, 0.066) | 0.197<br>(0.194, 0.200) | 0.392<br>(0.388, 0.395) | 0.169<br>(0.167, 0.171) | 0.366<br>(0.362, 0.369) | 0.589<br>(0.584, 0.594) |
| MANIQA | **-0.107**<br>(-0.108, -0.106) | **-0.221**<br>(-0.223, -0.219) | **-0.318**<br>(-0.322, -0.315) | -0.037<br>(-0.037, -0.036) | **-0.099**<br>(-0.1, -0.098) | **-0.187**<br>(-0.189, -0.184) | -0.0<br>(-0.0, -0.0) | **-0.002**<br>(-0.002, -0.001) | **-0.001**<br>(-0.001, -0.0) |

Table 6: All datasets, with domain transform, Abs. gain. Table 1

| Attack | FGSM | I-FGSM | MI-FGSM | AMI-FGSM | MADC | Korhonen et al. |
|---|---|---|---|---|---|---|
| CLIP-IQA | 0.243<br>(0.239, 0.248) | **0.484**<br>(0.476, 0.492) | **0.474**<br>(0.467, 0.482) | **0.471**<br>(0.464, 0.479) | 0.477<br>(0.469, 0.485) | 0.47<br>(0.463, 0.478) |
| META-IQA | 0.334<br>(0.328, 0.341) | 0.975<br>(0.968, 0.982) | 0.950<br>(0.943, 0.957) | 0.952<br>(0.945, 0.959) | 0.638<br>(0.632, 0.644) | 0.710<br>(0.704, 0.716) |
| RANK-IQA | 0.142<br>(0.136, 0.149) | 0.712<br>(0.707, 0.716) | 0.558<br>(0.555, 0.562) | 0.561<br>(0.557, 0.564) | **0.197**<br>(0.195, 0.2) | **0.43**<br>(0.425, 0.435) |
| HYPER-IQA | **-0.242**<br>(-0.251, -0.234) | 1.210<br>(1.199, 1.221) | 1.247<br>(1.236, 1.258) | 1.262<br>(1.251, 1.273) | 0.521<br>(0.515, 0.526) | 1.157<br>(1.147, 1.168) |
| KONCEPT | 0.314<br>(0.311, 0.318) | 0.940<br>(0.935, 0.945) | 0.701<br>(0.697, 0.706) | 0.702<br>(0.697, 0.706) | 0.416<br>(0.412, 0.420) | 0.671<br>(0.666, 0.676) |
| FPR | 0.490<br>(0.478, 0.503) | 6.078<br>(6.052, 6.104) | 5.713<br>(5.683, 5.742) | 5.724<br>(5.695, 5.753) | 1.864<br>(1.840, 1.888) | 5.246<br>(5.207, 5.284) |
| NIMA | 0.133<br>(0.128, 0.138) | 0.846<br>(0.839, 0.852) | 0.777<br>(0.770, 0.783) | 0.776<br>(0.770, 0.783) | 0.637<br>(0.630, 0.645) | 0.699<br>(0.691, 0.707) |
| WSP | 0.241<br>(0.238, 0.244) | 1.011<br>(1.004, 1.017) | 1.005<br>(0.999, 1.012) | 1.014<br>(1.007, 1.020) | 0.467<br>(0.462, 0.472) | 0.619<br>(0.614, 0.625) |
| MDTVSFA | 0.101<br>(0.095, 0.106) | 0.624<br>(0.618, 0.631) | 0.596<br>(0.59, 0.602) | 0.596<br>(0.59, 0.602) | 0.543<br>(0.537, 0.549) | 0.467<br>(0.462, 0.473) |
| LINEARITY | -0.098<br>(-0.103, -0.092) | 1.019<br>(1.013, 1.024) | 0.951<br>(0.947, 0.955) | 0.959<br>(0.955, 0.963) | 0.516<br>(0.511, 0.521) | 0.941<br>(0.936, 0.945) |
| VSFA | 0.173<br>(0.168, 0.178) | 2.439<br>(2.428, 2.451) | 2.901<br>(2.890, 2.912) | 2.905<br>(2.894, 2.917) | 1.392<br>(1.382, 1.403) | 1.596<br>(1.579, 1.614) |
| PAQ2PIQ | 0.319<br>(0.315, 0.322) | 0.860<br>(0.852, 0.868) | 0.782<br>(0.774, 0.789) | 0.783<br>(0.776, 0.791) | 0.274<br>(0.269, 0.278) | 0.640<br>(0.635, 0.646) |
| SPAQ | 0.163<br>(0.159, 0.167) | 1.374<br>(1.366, 1.381) | 1.171<br>(1.164, 1.177) | 1.176<br>(1.169, 1.183) | 0.476<br>(0.472, 0.481) | 1.092<br>(1.085, 1.099) |
| TRES | 0.479<br>(0.474, 0.485) | 0.903<br>(0.897, 0.909) | 0.878<br>(0.872, 0.884) | 0.880<br>(0.874, 0.886) | 0.448<br>(0.444, 0.453) | 0.848<br>(0.842, 0.855) |
| MANIQA | 0.295<br>(0.290, 0.299) | 1.325<br>(1.305, 1.344) | 0.939<br>(0.930, 0.948) | 0.942<br>(0.932, 0.951) | 0.412<br>(0.408, 0.416) | 0.529<br>(0.524, 0.535) |

Table 7: All datasets, with domain transform, Abs. gain. Table 2

| Attack | Optimized-UAP | | | Generative-UAP | | | Cumulative-UAP | | |
|---|---|---|---|---|---|---|---|---|---|
| Amplitude | 0.2 | 0.4 | 0.8 | 0.2 | 0.4 | 0.8 | 0.2 | 0.4 | 0.8 |
| CLIP-IQA | 0.078 (0.076, 0.080) | 0.272 (0.268, 0.277) | 0.329 (0.324, 0.334) | 0.017 (0.015, 0.019) | 0.169 (0.166, 0.172) | 0.298 (0.294, 0.303) | 0.008 (0.007, 0.008) | 0.028 (0.027, 0.029) | 0.081 (0.080, 0.083) |
| META-IQA | -0.013 (-0.014, -0.011) | 0.087 (0.083, 0.091) | 0.342 (0.335, 0.349) | -0.009 (-0.010, -0.009) | -0.01 (-0.012, -0.009) | 0.081 (0.078, 0.085) | 0.0 (0.0, 0.001) | 0.001 (0.001, 0.001) | 0.003 (0.002, 0.003) |
| RANK-IQA | -0.009 (-0.010, -0.007) | 0.101 (0.098, 0.103) | 0.221 (0.218, 0.225) | -0.01 (-0.011, -0.01) | 0.013 (0.012, 0.015) | 0.106 (0.103, 0.109) | 0.010 (0.010, 0.011) | 0.061 (0.059, 0.063) | 0.128 (0.125, 0.131) |
| HYPER-IQA | -0.052 (-0.054, -0.051) | 0.022 (0.019, 0.025) | 0.105 (0.1, 0.109) | **-0.033** (-0.034, -0.032) | -0.027 (-0.028, -0.026) | 0.05 (0.047, 0.053) | **-0.034** (-0.036, -0.033) | 0.032 (0.029, 0.035) | 0.132 (0.127, 0.137) |
| KONCEPT | 0.023 (0.021, 0.025) | 0.170 (0.166, 0.173) | 0.410 (0.404, 0.415) | -0.007 (-0.007, -0.006) | 0.074 (0.072, 0.077) | 0.239 (0.235, 0.243) | 0.037 (0.036, 0.039) | 0.172 (0.168, 0.176) | 0.347 (0.342, 0.351) |
| FPR | 0.435 (0.423, 0.448) | 1.717 (1.679, 1.755) | 5.305 (5.209, 5.402) | 0.102 (0.099, 0.104) | 0.463 (0.452, 0.474) | 1.250 (1.227, 1.272) | 0.153 (0.148, 0.159) | 0.765 (0.739, 0.791) | 2.441 (2.372, 2.511) |
| NIMA | -0.005 (-0.006, -0.004) | -0.003 (-0.005, -0.002) | 0.018 (0.016, 0.02) | 0.004 (0.004, 0.005) | 0.017 (0.016, 0.018) | 0.041 (0.039, 0.043) | 0.003 (0.002, 0.003) | 0.008 (0.007, 0.008) | 0.015 (0.014, 0.016) |
| WSP | 0.100 (0.097, 0.104) | 0.445 (0.436, 0.454) | 0.940 (0.927, 0.953) | 0.025 (0.024, 0.025) | 0.065 (0.063, 0.067) | 0.205 (0.200, 0.209) | 0.001 (0.001, 0.001) | 0.005 (0.004, 0.005) | 0.012 (0.012, 0.013) |
| MDTVSFA | 0.149 (0.145, 0.153) | 0.309 (0.304, 0.314) | 0.388 (0.384, 0.393) | 0.023 (0.022, 0.024) | 0.135 (0.132, 0.138) | 0.254 (0.250, 0.258) | 0.001 (0.001, 0.001) | 0.002 (0.002, 0.002) | 0.004 (0.004, 0.004) |
| LINEARITY | 0.229 (0.223, 0.235) | 0.567 (0.558, 0.577) | 0.970 (0.960, 0.981) | 0.024 (0.023, 0.026) | 0.192 (0.188, 0.197) | 0.393 (0.386, 0.399) | 0.204 (0.199, 0.210) | 0.520 (0.512, 0.529) | 0.903 (0.893, 0.914) |
| VSFA | 0.201 (0.195, 0.208) | 0.862 (0.846, 0.878) | 1.784 (1.766, 1.803) | 0.021 (0.020, 0.022) | 0.174 (0.169, 0.178) | 0.460 (0.452, 0.468) | 0.001 (0.001, 0.001) | 0.005 (0.005, 0.006) | 0.018 (0.017, 0.019) |
| PAQ2PIQ | 0.111 (0.108, 0.115) | 0.435 (0.428, 0.442) | 0.778 (0.770, 0.786) | -0.000 (-0.000, 0.000) | 0.093 (0.090, 0.096) | 0.345 (0.339, 0.350) | 0.094 (0.091, 0.098) | 0.384 (0.377, 0.390) | 0.703 (0.695, 0.710) |
| SPAQ | 0.010 (0.008, 0.012) | 0.438 (0.425, 0.452) | 1.458 (1.427, 1.489) | 0.025 (0.024, 0.026) | 0.173 (0.168, 0.179) | 0.472 (0.462, 0.482) | 0.002 (0.000, 0.004) | 0.392 (0.379, 0.405) | 1.439 (1.408, 1.471) |
| TRES | 0.144 (0.142, 0.147) | 0.288 (0.284, 0.291) | 0.445 (0.441, 0.450) | 0.046 (0.045, 0.046) | 0.140 (0.138, 0.142) | 0.279 (0.275, 0.283) | 0.120 (0.118, 0.122) | 0.260 (0.257, 0.264) | 0.416 (0.412, 0.420) |
| MANIQA | **-0.074** (-0.075, -0.073) | **-0.151** (-0.152, -0.15) | **-0.214** (-0.216, -0.212) | -0.026 (-0.026, -0.025) | **-0.069** (-0.07, -0.068) | **-0.128** (-0.129, -0.126) | -0.0 (-0.0, -0.0) | **-0.001** (-0.001, -0.001) | **-0.001** (-0.001, -0.0) |

Table 8: All datasets, with domain transform, Rel. gain. Table 1

| Attack | FGSM | I-FGSM | MI-FGSM | AMI-FGSM | MADC | Korhonen et al. |
|---|---|---|---|---|---|---|
| CLIP-IQA | 0.171<br>(0.167, 0.175) | **0.35**<br>(0.342, 0.358) | **0.344**<br>(0.336, 0.351) | **0.341**<br>(0.334, 0.349) | 0.344<br>(0.337, 0.352) | 0.339<br>(0.332, 0.347) |
| META-IQA | 0.251<br>(0.245, 0.256) | 0.736<br>(0.727, 0.744) | 0.716<br>(0.708, 0.725) | 0.718<br>(0.710, 0.727) | 0.478<br>(0.472, 0.484) | 0.529<br>(0.523, 0.536) |
| RANK-IQA | 0.100<br>(0.095, 0.104) | 0.45<br>(0.445, 0.455) | 0.352<br>(0.348, 0.356) | 0.354<br>(0.35, 0.357) | **0.128**<br>(0.125, 0.13) | **0.276**<br>(0.272, 0.281) |
| HYPER-IQA | **-0.146**<br>(-0.152, -0.141) | 0.758<br>(0.750, 0.766) | 0.784<br>(0.776, 0.792) | 0.791<br>(0.783, 0.799) | 0.335<br>(0.330, 0.340) | 0.728<br>(0.721, 0.736) |
| KONCEPT | 0.215<br>(0.212, 0.218) | 0.636<br>(0.631, 0.642) | 0.478<br>(0.473, 0.482) | 0.478<br>(0.473, 0.483) | 0.287<br>(0.283, 0.291) | 0.459<br>(0.454, 0.463) |
| FPR | 0.307<br>(0.300, 0.315) | 3.986<br>(3.961, 4.011) | 3.737<br>(3.714, 3.761) | 3.746<br>(3.723, 3.770) | 1.258<br>(1.237, 1.279) | 3.444<br>(3.414, 3.474) |
| NIMA | 0.093<br>(0.089, 0.097) | 0.564<br>(0.557, 0.571) | 0.517<br>(0.511, 0.524) | 0.517<br>(0.511, 0.524) | 0.425<br>(0.418, 0.432) | 0.468<br>(0.461, 0.475) |
| WSP | 0.171<br>(0.168, 0.174) | 0.714<br>(0.707, 0.721) | 0.709<br>(0.702, 0.715) | 0.716<br>(0.709, 0.723) | 0.337<br>(0.332, 0.342) | 0.439<br>(0.434, 0.445) |
| MDTVSFA | 0.069<br>(0.065, 0.073) | 0.412<br>(0.406, 0.418) | 0.394<br>(0.388, 0.401) | 0.394<br>(0.388, 0.4) | 0.360<br>(0.354, 0.366) | 0.307<br>(0.302, 0.312) |
| LINEARITY | -0.055<br>(-0.058, -0.052) | 0.651<br>(0.645, 0.657) | 0.604<br>(0.600, 0.609) | 0.608<br>(0.604, 0.613) | 0.336<br>(0.331, 0.340) | 0.598<br>(0.593, 0.603) |
| VSFA | 0.117<br>(0.114, 0.121) | 1.643<br>(1.633, 1.654) | 1.959<br>(1.946, 1.972) | 1.963<br>(1.950, 1.975) | 0.943<br>(0.934, 0.952) | 1.055<br>(1.043, 1.066) |
| PAQ2PIQ | 0.206<br>(0.202, 0.209) | 0.554<br>(0.546, 0.562) | 0.504<br>(0.496, 0.511) | 0.504<br>(0.497, 0.511) | 0.18<br>(0.176, 0.184) | 0.411<br>(0.406, 0.417) |
| SPAQ | 0.120<br>(0.117, 0.123) | 1.038<br>(1.029, 1.047) | 0.882<br>(0.874, 0.889) | 0.885<br>(0.878, 0.893) | 0.364<br>(0.359, 0.369) | 0.821<br>(0.814, 0.828) |
| TRES | 0.343<br>(0.338, 0.348) | 0.632<br>(0.625, 0.639) | 0.613<br>(0.607, 0.620) | 0.615<br>(0.609, 0.622) | 0.315<br>(0.311, 0.320) | 0.596<br>(0.589, 0.602) |
| MANIQA | 0.215<br>(0.211, 0.219) | 0.954<br>(0.938, 0.970) | 0.678<br>(0.669, 0.687) | 0.680<br>(0.671, 0.689) | 0.299<br>(0.295, 0.303) | 0.385<br>(0.380, 0.390) |

Table 9: All datasets, with domain transform, Rel. gain. Table 2

| Attack Amplitude | Optimized-UAP 0.2 | Optimized-UAP 0.4 | Optimized-UAP 0.8 | Generative-UAP 0.2 | Generative-UAP 0.4 | Generative-UAP 0.8 | Cumulative-UAP 0.2 | Cumulative-UAP 0.4 | Cumulative-UAP 0.8 |
|---|---|---|---|---|---|---|---|---|---|
| CLIP-IQA | 0.948 (0.935, 0.961) | 0.359 (0.350, 0.368) | 0.242 (0.235, 0.249) | 1.144 (1.130, 1.157) | 0.555 (0.545, 0.564) | 0.274 (0.267, 0.281) | 1.840 (1.826, 1.854) | 1.331 (1.318, 1.343) | 0.897 (0.886, 0.908) |
| META-IQA | 1.305 (1.291, 1.319) | 0.871 (0.857, 0.884) | 0.299 (0.289, 0.310) | 1.723 (1.709, 1.737) | 1.376 (1.363, 1.39) | 0.918 (0.904, 0.932) | 2.641 (2.625, 2.657) | 2.517 (2.502, 2.532) | **2.332** (2.318, 2.347) |
| RANK-IQA | 1.152 (1.140, 1.163) | 0.812 (0.799, 0.826) | 0.381 (0.372, 0.39) | 1.556 (1.544, 1.568) | 1.207 (1.195, 1.22) | 0.780 (0.767, 0.793) | 1.653 (1.639, 1.667) | 1.086 (1.071, 1.100) | 0.652 (0.641, 0.662) |
| HYPER-IQA | 0.996 (0.984, 1.007) | 1.007 (0.994, 1.02) | 0.692 (0.678, 0.705) | 1.282 (1.270, 1.294) | 1.188 (1.175, 1.200) | 1.014 (0.999, 1.028) | 1.149 (1.137, 1.160) | 1.055 (1.042, 1.069) | 0.632 (0.619, 0.645) |
| KONCEPT | 1.219 (1.206, 1.233) | 0.567 (0.555, 0.579) | 0.121 (0.111, 0.131) | 1.546 (1.534, 1.559) | 0.991 (0.977, 1.006) | 0.412 (0.400, 0.424) | 1.266 (1.252, 1.281) | 0.574 (0.562, 0.586) | 0.166 (0.158, 0.174) |
| FPR | 0.155 (0.145, 0.164) | -0.478 (-0.487, -0.469) | -1.019 (-1.026, -1.012) | 0.791 (0.781, 0.801) | 0.111 (0.102, 0.121) | -0.380 (-0.388, -0.373) | 0.648 (0.637, 0.659) | 0.004 (-0.008, 0.016) | -0.569 (-0.579, -0.558) |
| NIMA | **1.413** (1.4, 1.426) | **1.243** (1.23, 1.256) | **1.115** (1.103, 1.128) | 1.63 (1.616, 1.644) | **1.381** (1.368, 1.395) | **1.141** (1.128, 1.155) | 2.188 (2.173, 2.204) | 1.859 (1.844, 1.875) | 1.574 (1.559, 1.589) |
| WSP | 0.998 (0.983, 1.013) | 0.239 (0.225, 0.252) | -0.211 (-0.220, -0.203) | 1.517 (1.504, 1.531) | 1.117 (1.103, 1.130) | 0.575 (0.562, 0.587) | 2.404 (2.390, 2.417) | 2.157 (2.143, 2.171) | 1.834 (1.820, 1.849) |
| MDTVSFA | 0.706 (0.691, 0.721) | 0.267 (0.256, 0.277) | 0.094 (0.088, 0.100) | 1.396 (1.382, 1.411) | 0.735 (0.721, 0.749) | 0.337 (0.327, 0.347) | **2.853** (2.839, 2.866) | **2.581** (2.566, 2.595) | 2.267 (2.253, 2.282) |
| LINEARITY | 0.586 (0.570, 0.602) | 0.035 (0.023, 0.046) | -0.293 (-0.300, -0.287) | 1.393 (1.379, 1.408) | 0.647 (0.631, 0.662) | 0.190 (0.179, 0.202) | 0.648 (0.632, 0.664) | 0.078 (0.066, 0.089) | -0.260 (-0.267, -0.254) |
| VSFA | 0.646 (0.631, 0.662) | -0.094 (-0.107, -0.081) | -0.555 (-0.561, -0.548) | 1.364 (1.350, 1.378) | 0.675 (0.660, 0.689) | 0.139 (0.128, 0.150) | 2.512 (2.498, 2.526) | 2.241 (2.225, 2.257) | 1.890 (1.872, 1.908) |
| PAQ2PIQ | 0.986 (0.969, 1.003) | 0.101 (0.092, 0.110) | -0.229 (-0.233, -0.224) | **1.972** (1.958, 1.985) | 0.986 (0.971, 1.002) | 0.203 (0.194, 0.211) | 1.045 (1.028, 1.062) | 0.161 (0.152, 0.171) | -0.181 (-0.186, -0.176) |
| SPAQ | 1.314 (1.3, 1.327) | 0.409 (0.394, 0.424) | -0.160 (-0.175, -0.145) | 1.584 (1.570, 1.599) | 0.829 (0.814, 0.844) | 0.292 (0.279, 0.306) | 1.356 (1.343, 1.370) | 0.447 (0.432, 0.462) | -0.144 (-0.159, -0.129) |
| TRES | 0.586 (0.578, 0.594) | 0.247 (0.242, 0.252) | 0.031 (0.028, 0.035) | 1.110 (1.100, 1.119) | 0.604 (0.595, 0.612) | 0.265 (0.260, 0.271) | 0.684 (0.675, 0.693) | 0.300 (0.294, 0.306) | 0.066 (0.062, 0.070) |
| MANIQA | 0.861 (0.853, 0.870) | 0.524 (0.517, 0.531) | 0.374 (0.365, 0.383) | 1.359 (1.349, 1.368) | 0.900 (0.892, 0.909) | 0.622 (0.613, 0.631) | 2.532 (2.52, 2.545) | 2.405 (2.392, 2.418) | 2.158 (2.144, 2.172) |

Table 10: All datasets, with domain transform, Robustness score. Table 1

| Attack | FGSM | I-FGSM | MI-FGSM | AMI-FGSM | MADC | Korhonen et al. |
|---|---|---|---|---|---|---|
| CLIP-IQA | 0.532 (0.520, 0.544) | **0.21** (0.201, 0.219) | **0.219** (0.21, 0.229) | **0.221** (0.212, 0.231) | 0.216 (0.206, 0.225) | **0.22** (0.21, 0.229) |
| META-IQA | 0.400 (0.387, 0.412) | -0.140 (-0.144, -0.137) | -0.129 (-0.132, -0.125) | -0.130 (-0.133, -0.126) | 0.048 (0.044, 0.053) | 0.002 (-0.003, 0.006) |
| RANK-IQA | 0.712 (0.695, 0.730) | -0.019 (-0.023, -0.014) | 0.085 (0.081, 0.089) | 0.083 (0.079, 0.087) | **0.567** (0.559, 0.575) | 0.219 (0.212, 0.226) |
| HYPER-IQA | 0.579 (0.560, 0.597) | -0.243 (-0.247, -0.239) | -0.262 (-0.266, -0.258) | -0.265 (-0.269, -0.260) | 0.128 (0.122, 0.134) | -0.226 (-0.230, -0.221) |
| KONCEPT | 0.328 (0.321, 0.335) | -0.173 (-0.176, -0.170) | -0.045 (-0.049, -0.041) | -0.045 (-0.049, -0.041) | 0.194 (0.189, 0.200) | -0.023 (-0.027, -0.019) |
| FPR | 0.195 (0.180, 0.209) | -0.988 (-0.991, -0.985) | -0.960 (-0.963, -0.957) | -0.961 (-0.965, -0.958) | -0.446 (-0.453, -0.440) | -0.917 (-0.921, -0.913) |
| NIMA | 0.769 (0.752, 0.786) | -0.114 (-0.119, -0.109) | -0.076 (-0.080, -0.071) | -0.076 (-0.081, -0.071) | 0.027 (0.020, 0.033) | -0.015 (-0.022, -0.008) |
| WSP | 0.472 (0.464, 0.480) | -0.182 (-0.186, -0.178) | -0.180 (-0.183, -0.176) | -0.183 (-0.187, -0.179) | 0.166 (0.162, 0.171) | 0.040 (0.035, 0.045) |
| MDTVSFA | **0.808** (0.791, 0.825) | 0.045 (0.039, 0.051) | 0.067 (0.061, 0.073) | 0.067 (0.061, 0.073) | 0.113 (0.106, 0.120) | 0.18 (0.173, 0.188) |
| LINEARITY | 0.786 (0.771, 0.801) | -0.165 (-0.169, -0.161) | -0.137 (-0.141, -0.134) | -0.140 (-0.144, -0.136) | 0.143 (0.138, 0.149) | -0.130 (-0.134, -0.126) |
| VSFA | 0.698 (0.681, 0.716) | -0.573 (-0.576, -0.569) | -0.649 (-0.652, -0.645) | -0.650 (-0.653, -0.646) | -0.320 (-0.325, -0.316) | -0.359 (-0.367, -0.350) |
| PAQ2PIQ | 0.351 (0.346, 0.357) | -0.091 (-0.096, -0.087) | -0.051 (-0.055, -0.046) | -0.051 (-0.055, -0.046) | 0.428 (0.421, 0.435) | 0.034 (0.030, 0.039) |
| SPAQ | 0.718 (0.703, 0.733) | -0.296 (-0.300, -0.293) | -0.227 (-0.230, -0.224) | -0.229 (-0.233, -0.226) | 0.177 (0.172, 0.182) | -0.195 (-0.199, -0.192) |
| TRES | 0.163 (0.156, 0.171) | -0.136 (-0.140, -0.132) | -0.125 (-0.129, -0.120) | -0.125 (-0.130, -0.121) | 0.180 (0.174, 0.186) | -0.106 (-0.110, -0.101) |
| MANIQA | 0.409 (0.399, 0.419) | -0.277 (-0.283, -0.272) | -0.143 (-0.147, -0.139) | -0.144 (-0.148, -0.140) | 0.219 (0.215, 0.224) | 0.115 (0.110, 0.121) |

Table 11: All datasets, with domain transform, Robustness score. Table 2

| Attack | Optimized-UAP | | | Generative-UAP | | | Cumulative-UAP | | |
|---|---|---|---|---|---|---|---|---|---|
| Amplitude | 0.2 | 0.4 | 0.8 | 0.2 | 0.4 | 0.8 | 0.2 | 0.4 | 0.8 |
| CLIP-IQA | 0.107 | 0.377 | 0.456 | 0.021 | 0.240 | 0.416 | 0.011 | 0.041 | 0.116 |
| META-IQA | -0.020 | 0.110 | 0.451 | -0.013 | -0.016 | 0.104 | 0.001 | 0.001 | 0.004 |
| RANK-IQA | -0.041 | 0.149 | 0.342 | -0.020 | 0.035 | 0.157 | 0.017 | 0.090 | 0.192 |
| HYPER-IQA | -0.086 | 0.035 | 0.155 | **-0.052** | -0.048 | 0.065 | **-0.058** | 0.040 | 0.193 |
| KONCEPT | 0.030 | 0.241 | 0.594 | -0.011 | 0.104 | 0.342 | 0.052 | 0.245 | 0.501 |
| FPR | 0.621 | 2.502 | 7.970 | 0.146 | 0.665 | 1.836 | 0.218 | 1.093 | 3.657 |
| NIMA | -0.012 | -0.011 | 0.024 | 0.009 | 0.025 | 0.057 | 0.004 | 0.011 | 0.021 |
| WSP | 0.129 | 0.595 | 1.288 | 0.033 | 0.086 | 0.269 | 0.002 | 0.006 | 0.017 |
| MDTVSFA | 0.216 | 0.461 | 0.586 | 0.034 | 0.201 | 0.380 | 0.001 | 0.003 | 0.006 |
| LINEARITY | 0.333 | 0.859 | 1.500 | 0.032 | 0.281 | 0.591 | 0.296 | 0.786 | 1.393 |
| VSFA | 0.281 | 1.247 | 2.622 | 0.030 | 0.246 | 0.662 | 0.002 | 0.008 | 0.025 |
| PAQ2PIQ | 0.161 | 0.662 | 1.204 | -0.003 | 0.136 | 0.520 | 0.136 | 0.581 | 1.088 |
| SPAQ | 0.017 | 0.519 | 1.797 | 0.030 | 0.206 | 0.580 | -0.013 | 0.462 | 1.772 |
| TRES | 0.203 | 0.403 | 0.631 | 0.065 | 0.197 | 0.392 | 0.169 | 0.366 | 0.589 |
| MANIQA | **-0.107** | **-0.221** | **-0.318** | -0.037 | **-0.099** | **-0.187** | -0.001 | **-0.002** | **-0.002** |

Table 12: All datasets, with domain transform, Wasserstein score. Table 1

| Attack | FGSM | I-FGSM | MI-FGSM | AMI-FGSM | MADC | Korhonen et al. |
|---|---|---|---|---|---|---|
| CLIP-IQA | 0.243 | **0.484** | **0.474** | **0.471** | 0.477 | 0.470 |
| META-IQA | 0.334 | 0.975 | 0.950 | 0.952 | 0.638 | 0.710 |
| RANK-IQA | 0.142 | 0.712 | 0.558 | 0.561 | **0.197** | **0.430** |
| HYPER-IQA | **-0.243** | 1.210 | 1.247 | 1.262 | 0.521 | 1.157 |
| KONCEPT | 0.314 | 0.940 | 0.701 | 0.702 | 0.416 | 0.671 |
| FPR | 0.496 | 6.078 | 5.713 | 5.724 | 1.864 | 5.246 |
| NIMA | 0.133 | 0.846 | 0.777 | 0.776 | 0.637 | 0.699 |
| WSP | 0.241 | 1.011 | 1.005 | 1.014 | 0.467 | 0.619 |
| MDTVSFA | 0.101 | 0.624 | 0.596 | 0.596 | 0.543 | 0.467 |
| LINEARITY | -0.113 | 1.019 | 0.951 | 0.959 | 0.516 | 0.941 |
| VSFA | 0.173 | 2.439 | 2.901 | 2.905 | 1.392 | 1.596 |
| PAQ2PIQ | 0.319 | 0.860 | 0.782 | 0.783 | 0.274 | 0.640 |
| SPAQ | 0.163 | 1.374 | 1.171 | 1.176 | 0.476 | 1.092 |
| TRES | 0.479 | 0.903 | 0.878 | 0.880 | 0.448 | 0.848 |
| MANIQA | 0.295 | 1.325 | 0.939 | 0.942 | 0.412 | 0.529 |

Table 13: All datasets, with domain transform, Wasserstein score. Table 2

| metric | Cumulative-UAP COCO | Cumulative-UAP Pascal VOC 2012 | Generative-UAP COCO | Generative-UAP Pascal VOC 2012 | Optimized-UAP COCO | Optimized-UAP Pascal VOC 2012 |
|---|---|---|---|---|---|---|
| CLIP-IQA | 0.059 | 0.076 | 0.473 | 0.326 | 0.643 | 0.623 |
| META-IQA | 0.003 | 0.003 | -0.027 | -0.031 | 0.210 | 0.157 |
| RANK-IQA | 0.147 | 0.216 | 0.066 | 0.063 | 0.301 | 0.289 |
| HYPER-IQA | 0.108 | 0.074 | -0.092 | -0.097 | 0.083 | 0.069 |
| KONCEPT | 0.447 | 0.424 | 0.179 | 0.194 | 0.434 | 0.406 |
| FPR | 0.923 | 1.013 | 0.859 | 0.834 | 1.688 | 1.726 |
| NIMA | 0.014 | 0.023 | 0.030 | 0.065 | -0.022 | -0.027 |
| WSP | 0.006 | 0.018 | 0.126 | 0.184 | 0.775 | 0.798 |
| MDTVSFA | 0.004 | 0.006 | 0.319 | 0.404 | 0.756 | 0.755 |
| LINEARITY | 0.975 | 0.971 | 0.420 | 0.472 | 1.004 | 1.043 |
| VSFA | 0.004 | 0.024 | 0.330 | 0.394 | 1.174 | 1.130 |
| PAQ2PIQ | 0.866 | 0.883 | 0.234 | 0.270 | 0.948 | 0.941 |
| SPAQ | 0.568 | 0.551 | 0.406 | 0.313 | 0.647 | 0.564 |
| TRES | 0.627 | 0.643 | 0.358 | 0.359 | 0.697 | 0.686 |
| MANIQA | **-0.002** | **-0.005** | **-0.170** | **-0.179** | **-0.398** | **-0.382** |

Table 14: All datasets, with domain transform, Energy score, UAP attacks by dataset.

| Score Metric | $Abs.gain \downarrow$ | $Rel.gain \downarrow$ | $R_{score} \uparrow$ | $E_{score} \downarrow$ | $W_{score} \downarrow$ |
|---|---|---|---|---|---|
| CLIP-IQA | 0.272(0.270, 0.274) | 0.200(0.199, 0.202) | 0.705(0.700, 0.710) | 0.440 | 0.272 |
| META-IQA | 0.263(0.260, 0.266) | 0.206(0.204, 0.208) | **1.311(1.302, 1.319)** | 0.344 | 0.263 |
| RANK-IQA | 0.190(0.188, 0.192) | 0.125(0.124, 0.127) | 0.811(0.806, 0.815) | 0.295 | 0.190 |
| HYPER-IQA | 0.196(0.193, 0.199) | 0.117(0.116, 0.119) | 0.874(0.869, 0.879) | 0.253 | 0.199 |
| KONCEPT | 0.353(0.350, 0.355) | 0.241(0.240, 0.243) | 0.608(0.602, 0.613) | 0.495 | 0.353 |
| FPR | 2.874(2.846, 2.903) | 1.775(1.758, 1.793) | -0.165(-0.170, -0.160) | 1.424 | 2.874 |
| NIMA | 0.139(0.137, 0.141) | 0.092(0.091, 0.094) | 1.167(1.161, 1.172) | 0.215 | **0.139** |
| WSP | 0.332(0.329, 0.335) | 0.221(0.219, 0.223) | 1.018(1.011, 1.026) | 0.416 | 0.332 |
| MDTVSFA | 0.338(0.336, 0.340) | 0.230(0.228, 0.231) | 0.953(0.945, 0.962) | 0.494 | 0.338 |
| LINEARITY | 0.705(0.700, 0.709) | 0.452(0.449, 0.455) | 0.281(0.276, 0.286) | 0.783 | 0.705 |
| VSFA | 0.724(0.718, 0.730) | 0.474(0.470, 0.478) | 0.766(0.757, 0.775) | 0.675 | 0.724 |
| PAQ2PIQ | 0.504(0.501, 0.508) | 0.318(0.315, 0.320) | 0.516(0.511, 0.522) | 0.650 | 0.504 |
| SPAQ | 0.664(0.658, 0.671) | 0.504(0.499, 0.509) | 0.500(0.494, 0.506) | 0.632 | 0.664 |
| TRES | 0.555(0.552, 0.558) | 0.427(0.425, 0.430) | 0.295(0.292, 0.299) | 0.705 | 0.555 |
| MANIQA | **0.110(0.107, 0.114)** | **0.078(0.075, 0.080)** | 1.110(1.102, 1.118) | **0.206** | 0.175 |

Table 15: All datasets, all scores, without domain transform.

| Metric | CLIP-IQA | META-IQA | RANK-IQA | HYPER-IQA | KONCEPT | FPR | NIMA | WSP | MDTVSFA | LINEARITY | VSFA | PAQ2PIQ | SPAQ | TRES | MANIQA |
|---|---|---|---|---|---|---|---|---|---|---|---|---|---|---|---|
| CLIP-IQA | - | -1, 1, 1, 1, -1 | -1, 1, -1, -1, -1 | -1, 1, 1, 1, -1 | 1, 1, 1, -1, 1 | 1, 1, 1, 1, 1 | -1, 1, 1, 1, -1 | 1, 1, 1, -1, -1 | 1, 1, -, 1, -1 | 1, 1, 1, 1, 1 | 1, 1, 1, 1, 1 | 1, 1, 1, -1, 1 | 1, 1, 1, -, 1 | 1, 1, 1, -1, 1 | -1, 1, 1, -1, -1 |
| META-IQA | 1, -1, -1, -1, 1 | - | -1, -1, -1, -1, 1 | -1, 1, 1, -1, -1 | 1, -1, -1, -1, 1 | 1, 1, 1, 1, 1 | -1, -1, -, -, -1 | 1, 1, -1, -1, 1 | 1, -1, -1, -1, 1 | 1, -1, 1, -1, 1 | 1, 1, 1, 1, 1 | 1, -1, -1, -1, 1 | 1, 1, 1, -1, 1 | 1, -1, 1, -1, 1 | -1, 1, -1, -1, -1 |
| RANK-IQA | 1, -1, 1, 1, 1 | 1, 1, 1, 1, -1 | - | -1, 1, 1, 1, -1 | 1, 1, 1, 1, 1 | 1, 1, 1, 1, 1 | -1, 1, 1, 1, -1 | 1, 1, 1, 1, 1 | 1, -1, 1, 1, 1 | 1, 1, 1, 1, 1 | 1, 1, 1, 1, 1 | 1, 1, 1, 1, 1 | 1, 1, 1, 1, 1 | 1, 1, 1, 1, 1 | -1, 1, 1, 1, -1 |
| HYPER-IQA | 1, -1, -1, -1, 1 | 1, -1, -1, 1, 1 | 1, -1, -1, -1, 1 | - | 1, -1, -1, -1, 1 | 1, 1, 1, 1, 1 | -1, -1, -1, 1, 1 | 1, -1, -1, -1, 1 | 1, -1, -1, -, 1 | 1, -1, -1, -1, 1 | 1, 1, 1, 1, 1 | 1, -1, -1, -1, 1 | 1, 1, -1, -1, 1 | 1, -1, -1, -1, 1 | -1, -1, -1, -1, -1 |
| KONCEPT | -1, -1, -1, 1, -1 | -1, 1, 1, 1, -1 | -1, -1, -1, -1, -1 | -1, 1, 1, 1, -1 | - | 1, 1, 1, 1, 1 | -1, -1, 1, 1, -1 | 1, 1, -1, 1, -1 | -1, -1, -1, 1, -1 | 1, 1, 1, 1, 1 | 1, 1, 1, 1, 1 | 1, -1, -1, -1, 1 | 1, 1, 1, 1, 1 | 1, 1, 1, 1, 1 | -1, 1, -1, -, -1 |
| FPR | -1, -1, -1, -1, -1 | -1, -1, -1, -1, -1 | -1, -1, -1, -1, -1 | -1, -1, -1, -1, -1 | -1, -1, -1, -1, -1 | - | -1, -1, -1, -1, -1 | -1, -1, -1, -1, -1 | -1, -1, -1, -1, -1 | -1, -1, -1, -1, -1 | -1, -1, -1, -1, -1 | -1, -1, -1, -1, -1 | -1, -1, -1, -1, -1 | -1, -1, -1, -1, -1 | -1, -1, -1, -1, -1 |
| NIMA | 1, -1, -1, -1, 1 | 1, 1, -, -, 1 | 1, -1, -1, -1, 1 | 1, 1, 1, -1, -1 | 1, 1, -1, -1, 1 | 1, 1, 1, 1, 1 | - | 1, 1, -1, -1, 1 | 1, -1, -1, -1, 1 | 1, 1, 1, -1, 1 | 1, 1, 1, 1, 1 | 1, 1, -1, -1, 1 | 1, 1, 1, -1, 1 | 1, 1, 1, -1, 1 | -1, 1, -1, -1, -1 |
| WSP | -1, -1, -1, 1, 1 | -1, -1, 1, 1, -1 | -1, -1, -1, -1, -1 | -1, 1, 1, 1, -1 | -1, -1, 1, -1, 1 | 1, 1, 1, 1, 1 | -1, -1, 1, 1, -1 | - | -1, -1, -1, 1, -1 | 1, -1, 1, 1, 1 | 1, 1, 1, 1, 1 | 1, -1, -, -1, 1 | 1, 1, 1, 1, 1 | 1, -1, 1, -1, 1 | -1, 1, -1, -1, -1 |
| MDTVSFA | -1, -1, -, -1, 1 | -1, 1, 1, 1, -1 | -1, 1, -1, -1, -1 | -1, 1, 1, -, -1 | 1, 1, 1, -1, 1 | 1, 1, 1, 1, 1 | -1, 1, 1, 1, -1 | 1, 1, 1, -1, 1 | - | 1, 1, 1, -1, 1 | 1, 1, 1, 1, 1 | 1, 1, 1, -1, 1 | 1, 1, 1, -1, 1 | 1, 1, 1, -1, 1 | -1, 1, 1, -1, -1 |
| LINEARITY | -1, -1, -1, -1, -1 | -1, 1, -1, 1, -1 | -1, -1, -1, -1, -1 | -1, 1, 1, 1, -1 | -1, -1, -1, -1, -1 | 1, 1, 1, 1, 1 | -1, -1, -1, 1, -1 | -1, 1, -1, -1, -1 | -1, -1, -1, 1, -1 | - | 1, 1, 1, 1, -1 | -1, -1, -1, -1, -1 | -1, 1, 1, -1, -1 | -1, 1, -1, -1, -1 | -1, 1, -1, -1, -1 |
| VSFA | -1, -1, -1, -1, -1 | -1, -1, -1, -1, -1 | -1, -1, -1, -1, -1 | -1, -1, -1, -1, -1 | -1, -1, -1, -1, -1 | 1, 1, 1, 1, 1 | -1, -1, -1, -1, -1 | -1, -1, -1, -1, -1 | -1, -1, -1, -1, -1 | -1, -1, -1, -1, 1 | - | -1, -1, -1, -1, -1 | -1, -1, -1, -1, -1 | -1, -1, -1, -1, -1 | -1, -1, -1, -1, -1 |
| PAQ2PIQ | -1, -1, -1, 1, -1 | -1, 1, 1, 1, -1 | -1, -1, -1, -1, -1 | -1, 1, 1, 1, -1 | -1, 1, 1, 1, -1 | 1, 1, 1, 1, 1 | -1, -1, 1, 1, -1 | -1, 1, -, 1, -1 | -1, -1, -1, 1, -1 | 1, 1, 1, 1, 1 | 1, 1, 1, 1, 1 | - | 1, 1, 1, 1, -1 | -1, 1, 1, 1, -1 | -1, 1, -1, 1, -1 |
| SPAQ | -1, -1, -1, -, -1 | -1, -1, -1, 1, -1 | -1, -1, -1, -1, -1 | -1, -1, 1, 1, -1 | -1, -1, -1, -1, -1 | 1, 1, 1, 1, 1 | -1, -1, -1, 1, -1 | -1, -1, -1, -1, -1 | -1, -1, -1, 1, -1 | 1, -1, -1, 1, 1 | 1, 1, 1, 1, 1 | -1, -1, -1, -1, 1 | - | -1, -1, -1, -1, -1 | -1, -1, -1, -1, -1 |
| TRES | -1, -1, -1, 1, -1 | -1, 1, -1, 1, -1 | -1, -1, -1, -1, -1 | -1, 1, 1, 1, -1 | -1, -1, -1, -1, -1 | 1, 1, 1, 1, 1 | -1, -1, -1, 1, -1 | -1, 1, -1, 1, -1 | -1, -1, -1, 1, -1 | 1, -1, 1, 1, 1 | 1, 1, 1, 1, 1 | 1, -1, -1, -1, 1 | 1, 1, 1, 1, 1 | - | -1, 1, -1, -1, -1 |
| MANIQA | 1, -1, -1, 1, 1 | 1, -1, 1, 1, 1 | 1, -1, -1, -1, 1 | 1, 1, 1, 1, 1 | 1, -1, 1, -, 1 | 1, 1, 1, 1, 1 | 1, -1, 1, 1, 1 | 1, -1, 1, 1, 1 | 1, -1, -1, 1, 1 | 1, -1, 1, 1, 1 | 1, 1, 1, 1, 1 | 1, -1, 1, -1, 1 | 1, 1, 1, 1, 1 | 1, -1, 1, 1, 1 | - |

Table 16: Results of one-sided Wilcoxon rank-sum tests performed on Absolute gains for the metrics compared above. For each pair of metrics, the table shows values for different types of attacks in the following order: all attacks, FGSM-based, Korhonen-et-al, MADC, UAP-based. A value of 1 indicates the metric for that row is statistically superior to the metric for that column (its gains are lower than the gains of the metric in the column). A -1 value indicates the opposite. A hyphen (-) indicates they cannot be statistically distinguished with p-value $\leq 0.05$.
